# Supplementary material for: Synthesizing Images of Humans in Unseen Poses
Source: arXiv:1804.07739 source file (2018-04-20)
Supplement: Supplementary file 1 [file appendices.tex]

\begin{appendices}
\section{Network Architectures}
\label{sec:appendixA}
Let C$k$ denote a convolution layer with $k$ filters, C$k_2$ a convolution layer with stride 2, U a (2x) spatial upsampling layer, D$k$ a dense layer with $k$ filters and F a flattening layer. All convolution layers use a kernel size of $3$ except for the first convolution of the encoder of each UNet which uses a kernel size of $7$. Convolutions and dense layers are followed by a Leaky ReLU activation unless specified otherwise. All input volumes to the following networks have spatial resolution of $256x256$.

\subsection{Source Image Segmentation Network}
\noindent Input: $[I_s,p_s] \in \mathcal{R}^{256x256x17}$\\
Output: $M_s \in \mathcal{R}^{256x256x11}$\\
\\
\textbf{Encoder:}\\
C$64$, C$64_2$, C$128$, C$128_2$, C$128$, C$128_2$, C$128$, C$128_2$, C$128$, C$128_2$\\
\textbf{Decoder:}\\
C$128$,U, C$128$, U, C$128$, U, C$128$, U, C$128$, U, C$64$, C$11$\\
\\
Skip layers concatenate output volumes (after activation) of layers $1,3,5,7,9$ of the encoder to the outputs volumes (after activation) of layers $3,5,7,9,11$ of the decoder. The final convolution of the decoder, C$11$ is followed by a linear activation. 

\subsection{Background Synthesis Network}
\noindent Input: $[I_s,p_s] \in \mathcal{R}^{256x256x17}$\\
Output: $y_{bg} \in \mathcal{R}^{256x256x3}$\\
\\
This architecture is identical to the source image segmentation network, except that the final convolution, C$11$, is replaced by C$3$ and is followed by a \emph{tanh} activation.

\subsection{Foreground Synthesis Network}
\noindent Input: $[W,p_t] \in \mathcal{R}^{256x256x44}$\\
Output: $y_{fg} \in \mathcal{R}^{256x256x3}$, $M_t \in \mathcal{R}^{256x256x1}$\\
\\
\textbf{Encoder:}\\
C$128$, C$128_2$, C$128$, C$128_2$, C$256$, C$256_2$, C$256$, C$256_2$, C$256$, C$256_2$\\
\textbf{Decoder:}\\
C$256$,U, C$256$, U, C$256$, U, C$256$, U, C$128$, U, C$64$, C$3$/C$1$\\
\\
Skip layers concatenate output volumes (after activation) of layers $1,3,5,7,9$ of the encoder to the outputs volumes (after activation) of layers $3,5,7,9,11$ of the decoder. We have two separate convolutions as the final layers of the decoder, producing two outputs. The output of C$3$ is followed by a \emph{tanh} activation to yield $y_{fg}$. The output of C$1$ is followed by a $\emph{sigmoid}$ activation to produce $M_t$. 

\subsection{Discriminator Network}
\noindent Input: $[y,p_t] \in \mathcal{R}^{256x256x17}$\\
Output: $y_{class} \in \mathcal{R}^{2}$\\
C$64_2$, C$128_2$, C$256_2$, C$256_2$,C$256_2$,C$256$, F, D$256$, D$256$, D$2$\\
\\
The final dense layer uses a \emph{softmax} activation. 

\section{Additional Results}
We present additional results to show that our method is robust to a variety of appearances not shown in the initial results. Fig.~\ref{fig:extra_results} shows additional results using our different loss functions. Fig.~\ref{fig:extra_transfer_results} shows additional cross-action synthesized images. 

\begin{figure*}[h!]
\begin{center}
\includegraphics[width=\textwidth]{extra_results_images.pdf}
\end{center}
\caption{Additional outputs of our method for different loss functions.}
\label{fig:extra_results}
\end{figure*}

\begin{figure*}[h!]
\begin{center}
\includegraphics[scale=1.5]{extra_transfer_images.pdf}
\end{center}
\caption{Additional cross-action synthesis outputs of our method.}
\label{fig:extra_transfer_results}
\end{figure*}

%\section{Video Synthesis}
%We placed video sequences (golf\_sequence.mov and tennis\_sequence.mov) for the examples described in Sec.~\ref{videosynthesis}, in the zip file. We show the ground truth sequence, our synthesized sequence, and our synthesized target masks. We present the masks to show that our segmentations are also consistent over time.

\end{appendices}
